# Supplementary material for: Spin-Conserved and Spin-Flip Optical Excitations From the Bethe-Salpeter Equation Formalism
Source: arXiv:2101.08680 source file (2021-02-26)
Supplement: Supplementary file 1 [file sfBSE-SI.pdf]

# Supporting Information for “Spin-Conserved and Spin-Flip Optical Excitations From the Bethe-Salpeter Equation Formalism”

Enzo Monino<sup>1</sup> and Pierre-François Loos<sup>1, a)</sup>

*Laboratoire de Chimie et Physique Quantiques (UMR 5626), Université de Toulouse, CNRS, UPS, France*

TABLE I. Excitation energies with respect to the  $X^1\Sigma_g^+$  ground state of the  $B^1\Sigma_u^+$  and  $E^1\Sigma_g^+$  states of  $H_2$  obtained with the cc-pVQZ basis at the CIS, TD-BH&HLYP, BSE@ $G_0W_0$ , and EOM-CCSD levels of theory.

| $R(H-H)$ (Å) | CIS             |                 | BH&HLYP         |                 | BSE@ $G_0W_0$   |                 | EOM-CCSD        |                 |
|--------------|-----------------|-----------------|-----------------|-----------------|-----------------|-----------------|-----------------|-----------------|
|              | $B^1\Sigma_u^+$ | $E^1\Sigma_g^+$ | $B^1\Sigma_u^+$ | $E^1\Sigma_g^+$ | $B^1\Sigma_u^+$ | $E^1\Sigma_g^+$ | $B^1\Sigma_u^+$ | $E^1\Sigma_g^+$ |
| 0.5          | 15.942          | 17.398          | 15.253          | 16.896          | 15.535          | 16.135          | 15.703          | 16.737          |
| 0.6          | 14.791          | 16.579          | 14.18           | 16.199          | 14.767          | 15.073          | 14.61           | 16.056          |
| 0.7          | 13.745          | 15.891          | 13.339          | 15.614          | 14.108          | 14.12           | 13.621          | 15.491          |
| 0.8          | 12.8            | 15.311          | 12.514          | 15.122          | 13.236          | 13.591          | 12.735          | 15.017          |
| 0.9          | 11.943          | 14.815          | 11.766          | 14.699          | 12.444          | 13.126          | 11.938          | 14.615          |
| 1.           | 11.163          | 14.389          | 11.088          | 14.334          | 11.722          | 12.733          | 11.224          | 14.27           |
| 1.1          | 10.454          | 14.025          | 10.474          | 14.02           | 11.068          | 12.41           | 10.587          | 13.962          |
| 1.2          | 9.8096          | 13.712          | 9.919           | 13.75           | 10.477          | 12.132          | 10.023          | 13.648          |
| 1.3          | 9.3685          | 13.401          | 9.421           | 13.515          | 9.4696          | 12.139          | 9.5306          | 13.201          |
| 1.4          | 9.1278          | 13.262          | 8.9771          | 13.309          | 8.7427          | 12.211          | 9.1076          | 14.241          |
| 1.5          | 8.9859          | 13.18           | 8.5848          | 13.127          | 8.2988          | 12.3            | 8.7525          | 13.814          |
| 1.6          | 8.9106          | 13.125          | 8.2413          | 12.966          | 8.0543          | 12.395          | 8.4631          | 13.606          |
| 1.7          | 8.8839          | 13.085          | 7.9431          | 12.824          | 7.9457          | 12.482          | 8.2361          | 13.475          |
| 1.8          | 8.8936          | 13.058          | 7.6866          | 12.699          | 7.9282          | 12.563          | 8.0669          | 13.383          |
| 1.9          | 8.9307          | 13.041          | 7.4677          | 12.593          | 7.9697          | 12.641          | 7.9505          | 13.317          |
| 2.           | 8.9888          | 13.033          | 7.2827          | 12.502          | 8.0486          | 12.714          | 7.881           | 13.272          |
| 2.1          | 9.0627          | 13.031          | 7.1279          | 12.421          | 8.1508          | 12.783          | 7.8523          | 13.239          |
| 2.2          | 9.1485          | 13.031          | 6.9996          | 12.343          | 8.2671          | 12.845          | 7.8581          | 13.212          |
| 2.3          | 9.2429          | 13.031          | 6.8947          | 12.265          | 8.3914          | 12.901          | 7.8923          | 13.187          |
| 2.4          | 9.3435          | 13.031          | 6.81            | 12.186          | 8.5197          | 12.951          | 7.9492          | 13.164          |
| 2.5          | 9.4484          | 13.032          | 6.7427          | 12.109          | 8.6495          | 12.997          | 8.0239          | 13.145          |
| 2.6          | 9.5561          | 13.037          | 6.6902          | 12.03           | 8.7792          | 13.042          | 8.1122          | 13.133          |
| 2.7          | 9.6657          | 13.043          | 6.6501          | 11.946          | 8.908           | 13.084          | 8.2105          | 13.125          |
| 2.8          | 9.7763          | 13.05           | 6.6205          | 11.851          | 9.0353          | 13.123          | 8.3162          | 13.12           |
| 2.9          | 9.8874          | 13.056          | 6.5996          | 11.744          | 9.1605          | 13.154          | 8.4269          | 13.115          |
| 3.           | 9.9984          | 13.057          | 6.5857          | 11.627          | 9.283           | 13.174          | 8.5408          | 13.106          |
| 3.1          | 10.109          | 13.053          | 6.5778          | 11.505          | 9.4032          | 13.183          | 8.6564          | 13.091          |
| 3.2          | 10.219          | 13.043          | 6.5746          | 11.383          | 9.5211          | 13.181          | 8.7726          | 13.069          |
| 3.3          | 10.328          | 13.027          | 6.5754          | 11.266          | 9.6369          | 13.169          | 8.8884          | 13.041          |
| 3.4          | 10.435          | 13.006          | 6.5792          | 11.158          | 9.7506          | 13.15           | 9.003           | 13.008          |
| 3.5          | 10.541          | 12.983          | 6.5856          | 11.062          | 9.862           | 13.126          | 9.1159          | 12.972          |
| 3.6          | 10.645          | 12.958          | 6.5939          | 10.977          | 9.971           | 13.1            | 9.2265          | 12.935          |
| 3.7          | 10.748          | 12.933          | 6.6037          | 10.905          | 10.077          | 13.073          | 9.3347          | 12.899          |
| 3.8          | 10.848          | 12.908          | 6.6145          | 10.846          | 10.181          | 13.047          | 9.4401          | 12.863          |
| 3.9          | 10.947          | 12.884          | 6.626           | 10.798          | 10.282          | 13.023          | 9.5424          | 12.83           |
| 4.           | 11.043          | 12.861          | 6.6381          | 10.761          | 10.38           | 13.             | 9.6415          | 12.8            |

<sup>a)</sup>Electronic mail: [loos@irsamc.ups-tlse.fr](mailto:loos@irsamc.ups-tlse.fr)

TABLE II. Excitation energies with respect to the  $X^1\Sigma_g^+$  ground state of the  $B^1\Sigma_u^+$ ,  $E^1\Sigma_g^+$ , and  $F^1\Sigma_g^+$  states of  $H_2$  obtained with the cc-pVQZ basis at the SF-CIS, SF-TD-BH&HLYP, SF-BSE@ $G_0W_0$ , and EOM-CCSD levels of theory. All the spin-conserved and spin-flip calculations have been performed with an unrestricted reference.

| $R(H-H)$ (Å) | SF-CIS          |                 |                 | SF-BH&HLYP      |                 |                 | SF-BSE@ $G_0W_0$ |                 |                 | EOM-CCSD        |                 |                 |
|--------------|-----------------|-----------------|-----------------|-----------------|-----------------|-----------------|------------------|-----------------|-----------------|-----------------|-----------------|-----------------|
|              | $B^1\Sigma_u^+$ | $E^1\Sigma_g^+$ | $F^1\Sigma_g^+$ | $B^1\Sigma_u^+$ | $E^1\Sigma_g^+$ | $F^1\Sigma_g^+$ | $B^1\Sigma_u^+$  | $E^1\Sigma_g^+$ | $F^1\Sigma_g^+$ | $B^1\Sigma_u^+$ | $E^1\Sigma_g^+$ | $F^1\Sigma_g^+$ |
| 0.5          | 14.829          | 15.279          | 28.726          | 17.276          | 13.506          | 27.846          | 16.208           | 16.026          | 29.398          | 15.703          | 17.126          | 29.997          |
| 0.6          | 14.057          | 14.694          | 27.528          | 15.523          | 12.674          | 26.696          | 14.953           | 15.206          | 28.044          | 14.61           | 16.38           | 28.608          |
| 0.7          | 13.385          | 14.227          | 26.27           | 13.916          | 11.978          | 25.396          | 13.759           | 14.469          | 26.668          | 13.621          | 15.76           | 27.011          |
| 0.8          | 12.784          | 13.849          | 24.801          | 12.469          | 11.414          | 23.715          | 12.92            | 13.824          | 25.101          | 12.735          | 15.244          | 25.114          |
| 0.9          | 12.228          | 13.535          | 22.906          | 11.191          | 10.965          | 21.235          | 12.141           | 13.284          | 23.004          | 11.938          | 14.808          | 22.869          |
| 1.           | 11.71           | 13.273          | 20.834          | 10.086          | 10.617          | 18.824          | 11.434           | 12.849          | 20.725          | 11.224          | 14.437          | 20.591          |
| 1.1          | 11.233          | 13.054          | 18.885          | 9.1444          | 10.353          | 16.693          | 10.803           | 12.507          | 18.643          | 10.587          | 14.114          | 18.502          |
| 1.2          | 10.804          | 12.869          | 17.164          | 8.3499          | 10.155          | 14.838          | 10.246           | 12.241          | 16.776          | 10.023          | 13.811          | 16.68           |
| 1.3          | 10.427          | 12.704          | 15.7            | 7.6792          | 10.003          | 13.233          | 9.7563           | 12.023          | 15.185          | 9.5306          | 13.456          | 15.2            |
| 1.4          | 10.106          | 12.526          | 14.516          | 7.1116          | 9.8732          | 11.863          | 9.3359           | 11.821          | 13.884          | 9.1076          | 14.241          | 12.853          |
| 1.5          | 9.8431          | 12.262          | 13.663          | 6.6301          | 9.7087          | 10.751          | 8.9836           | 11.554          | 12.889          | 8.7525          | 13.814          | 11.971          |
| 1.6          | 9.6364          | 13.198          | 11.831          | 6.2217          | 10.108          | 9.2661          | 8.6957           | 12.31           | 11.105          | 8.4631          | 13.606          | 11.096          |
| 1.7          | 9.4831          | 13.006          | 11.32           | 5.8767          | 9.9322          | 8.5243          | 8.4675           | 12.066          | 10.52           | 8.2361          | 13.475          | 10.347          |
| 1.8          | 9.3786          | 12.933          | 10.855          | 5.5871          | 9.8777          | 7.8097          | 8.2964           | 11.962          | 9.9678          | 8.0669          | 13.383          | 9.7387          |
| 1.9          | 9.3173          | 12.913          | 10.481          | 5.3465          | 9.862           | 7.1894          | 8.1749           | 11.916          | 9.5101          | 7.9505          | 13.317          | 9.2619          |
| 2.           | 9.2934          | 12.922          | 10.197          | 5.1495          | 9.8671          | 6.6653          | 8.0991           | 11.902          | 9.152           | 7.881           | 13.272          | 8.9019          |
| 2.1          | 9.3009          | 12.943          | 9.9949          | 4.991           | 9.8815          | 6.2297          | 8.0645           | 11.903          | 8.8854          | 7.8523          | 13.239          | 8.642           |
| 2.2          | 9.3342          | 12.968          | 9.8615          | 4.8667          | 9.8946          | 5.8728          | 8.0632           | 11.908          | 8.6977          | 7.8581          | 13.212          | 8.4659          |
| 2.3          | 9.3878          | 12.988          | 9.7841          | 4.7722          | 9.9011          | 5.585           | 8.0893           | 11.911          | 8.5761          | 7.8923          | 13.187          | 8.3583          |
| 2.4          | 9.4572          | 13.005          | 9.7515          | 4.7034          | 9.9021          | 5.357           | 8.1373           | 11.915          | 8.5077          | 7.9492          | 13.164          | 8.3054          |
| 2.5          | 9.5384          | 12.987          | 9.7538          | 4.6565          | 9.9014          | 5.1798          | 8.2035           | 11.919          | 8.4827          | 8.0239          | 13.145          | 8.2956          |
| 2.6          | 9.6283          | 12.971          | 9.783           | 4.6277          | 9.9008          | 5.0451          | 8.2838           | 11.924          | 8.4919          | 8.1122          | 13.133          | 8.319           |
| 2.7          | 9.7245          | 12.968          | 9.8329          | 4.6139          | 9.8999          | 4.9458          | 8.3743           | 11.93           | 8.5274          | 8.2105          | 13.125          | 8.3677          |
| 2.8          | 9.825           | 12.972          | 9.8983          | 4.6124          | 9.8959          | 4.8758          | 8.473            | 11.933          | 8.5834          | 8.3162          | 13.12           | 8.4355          |
| 2.9          | 9.9281          | 12.979          | 9.9751          | 4.6208          | 9.8857          | 4.8292          | 8.5762           | 11.934          | 8.6537          | 8.4269          | 13.115          | 8.5173          |
| 3.           | 10.033          | 12.986          | 10.06           | 4.6369          | 9.8666          | 4.8016          | 8.6819           | 11.93           | 8.7342          | 8.5408          | 13.106          | 8.6091          |
| 3.1          | 10.139          | 12.989          | 10.152          | 4.6592          | 9.8385          | 4.7891          | 8.7879           | 11.921          | 8.8214          | 8.6564          | 13.091          | 8.7079          |
| 3.2          | 10.244          | 12.987          | 10.247          | 4.6864          | 9.803           | 4.7887          | 8.8935           | 11.905          | 8.9133          | 8.7726          | 13.069          | 8.8112          |
| 3.3          | 10.345          | 12.979          | 10.35           | 4.7174          | 9.7627          | 4.7978          | 8.9983           | 11.884          | 9.0085          | 8.8884          | 13.041          | 8.9172          |
| 3.4          | 10.445          | 12.966          | 10.454          | 4.7512          | 9.7205          | 4.8144          | 9.1033           | 11.857          | 9.1066          | 9.003           | 13.008          | 9.0243          |
| 3.5          | 10.546          | 12.949          | 10.558          | 4.7873          | 9.679           | 4.8368          | 9.2059           | 11.829          | 9.2071          | 9.1159          | 12.972          | 9.1315          |
| 3.6          | 10.646          | 12.93           | 10.66           | 4.8249          | 9.64            | 4.8636          | 9.3055           | 11.8            | 9.3098          | 9.2265          | 12.935          | 9.2378          |
| 3.7          | 10.746          | 12.91           | 10.76           | 4.8635          | 9.6045          | 4.8937          | 9.4048           | 11.771          | 9.4109          | 9.3347          | 12.899          | 9.3427          |
| 3.8          | 10.845          | 12.889          | 10.859          | 4.9029          | 9.5734          | 4.9265          | 9.5033           | 11.743          | 9.5104          | 9.4401          | 12.863          | 9.4455          |
| 3.9          | 10.942          | 12.868          | 10.956          | 4.9425          | 9.5465          | 4.9609          | 9.6003           | 11.717          | 9.6078          | 9.5424          | 12.83           | 9.546           |
| 4.           | 11.038          | 12.848          | 11.051          | 4.9822          | 9.5238          | 4.9964          | 9.6956           | 11.693          | 9.7031          | 9.6415          | 12.8            | 9.6437          |

TABLE III. Expectation value of the spin operator  $\langle \hat{S}^2 \rangle$  of the  $B^1\Sigma_u^+$ ,  $E^1\Sigma_g^+$ , and  $F^1\Sigma_g^+$  states of  $H_2$  obtained with the cc-pVQZ basis at the SF-CIS, SF-TD-BH&HLYP, SF-BSE@ $G_0W_0$ , and EOM-CCSD levels of theory. All the spin-conserved and spin-flip calculations have been performed with an unrestricted reference.

| $R(H-H)$ (Å) | SF-CIS          |                 |                 | SF-BH&HLYP      |                 |                 | SF-BSE@ $G_0W_0$ |                 |                 |
|--------------|-----------------|-----------------|-----------------|-----------------|-----------------|-----------------|------------------|-----------------|-----------------|
|              | $B^1\Sigma_u^+$ | $E^1\Sigma_g^+$ | $F^1\Sigma_g^+$ | $B^1\Sigma_u^+$ | $E^1\Sigma_g^+$ | $F^1\Sigma_g^+$ | $B^1\Sigma_u^+$  | $E^1\Sigma_g^+$ | $F^1\Sigma_g^+$ |
| 0.5          | 0.0472          | 0.9825          | 0.987           | 0.8926          | 0.9746          | 1.              | 0.1904           | 0.9774          | 0.9936          |
| 0.6          | 0.0735          | 0.9849          | 0.9664          | 0.8418          | 0.9734          | 1.              | 0.0716           | 0.9778          | 0.9827          |
| 0.7          | 0.1058          | 0.9875          | 0.9001          | 0.7782          | 0.972           | 0.9251          | 0.1123           | 0.9785          | 0.9262          |
| 0.8          | 0.1373          | 0.99            | 0.7033          | 0.694           | 0.9707          | 0.4824          | 0.1382           | 0.9796          | 0.7122          |
| 0.9          | 0.1623          | 0.992           | 0.4176          | 0.5923          | 0.9694          | 0.1771          | 0.1602           | 0.981           | 0.3645          |
| 1.           | 0.178           | 0.9932          | 0.2486          | 0.4851          | 0.9681          | 0.143           | 0.1736           | 0.9822          | 0.2031          |
| 1.1          | 0.1849          | 0.9928          | 0.1776          | 0.3875          | 0.9666          | 0.1412          | 0.1799           | 0.9827          | 0.1488          |
| 1.2          | 0.1853          | 0.9886          | 0.1528          | 0.3103          | 0.9645          | 0.1447          | 0.1785           | 0.9805          | 0.1316          |
| 1.3          | 0.1817          | 0.9731          | 0.1576          | 0.2555          | 0.9598          | 0.1509          | 0.1744           | 0.9708          | 0.1395          |
| 1.4          | 0.1763          | 0.9202          | 0.2082          | 0.2192          | 0.9432          | 0.1682          | 0.1689           | 0.9342          | 0.1753          |
| 1.5          | 0.1706          | 0.7566          | 0.3737          | 0.196           | 0.8475          | 0.2642          | 0.1639           | 0.7966          | 0.3175          |
| 1.6          | 0.1658          | 0.6399          | 0.4945          | 0.1816          | 0.6784          | 0.4335          | 0.1597           | 0.6174          | 0.5018          |
| 1.7          | 0.1623          | 0.807           | 0.3334          | 0.173           | 0.8802          | 0.2321          | 0.1571           | 0.8172          | 0.3083          |
| 1.8          | 0.1607          | 0.8814          | 0.2662          | 0.1684          | 0.9249          | 0.1883          | 0.1561           | 0.8959          | 0.237           |
| 1.9          | 0.161           | 0.9174          | 0.2381          | 0.1664          | 0.9409          | 0.174           | 0.1568           | 0.931           | 0.2097          |
| 2.           | 0.1631          | 0.9371          | 0.2268          | 0.1662          | 0.9488          | 0.1683          | 0.1589           | 0.9493          | 0.1996          |
| 2.1          | 0.1669          | 0.9488          | 0.2234          | 0.1674          | 0.9535          | 0.1663          | 0.1624           | 0.9596          | 0.1973          |
| 2.2          | 0.1722          | 0.9561          | 0.2245          | 0.1695          | 0.9567          | 0.1663          | 0.1672           | 0.9661          | 0.1989          |
| 2.3          | 0.1788          | 0.9606          | 0.2281          | 0.1723          | 0.9589          | 0.1677          | 0.1731           | 0.9704          | 0.2027          |
| 2.4          | 0.1866          | 0.9633          | 0.2333          | 0.1754          | 0.9604          | 0.1698          | 0.1797           | 0.9729          | 0.2078          |
| 2.5          | 0.1953          | 0.9645          | 0.2397          | 0.1789          | 0.9614          | 0.1726          | 0.187            | 0.9741          | 0.2138          |
| 2.6          | 0.2047          | 0.9643          | 0.2468          | 0.1826          | 0.9619          | 0.1758          | 0.1947           | 0.974           | 0.2205          |
| 2.7          | 0.2145          | 0.9627          | 0.2544          | 0.1864          | 0.9619          | 0.1793          | 0.2028           | 0.9727          | 0.2277          |
| 2.8          | 0.2247          | 0.9596          | 0.2623          | 0.1902          | 0.9614          | 0.183           | 0.2113           | 0.9699          | 0.2353          |
| 2.9          | 0.2349          | 0.9553          | 0.2704          | 0.1939          | 0.9605          | 0.1867          | 0.2201           | 0.9656          | 0.2435          |
| 3.           | 0.2451          | 0.9497          | 0.2783          | 0.1975          | 0.9593          | 0.1905          | 0.2293           | 0.96            | 0.2519          |
| 3.1          | 0.255           | 0.9431          | 0.286           | 0.201           | 0.9578          | 0.1942          | 0.2385           | 0.9538          | 0.2602          |
| 3.2          | 0.2646          | 0.936           | 0.2934          | 0.2042          | 0.956           | 0.1977          | 0.2475           | 0.9473          | 0.268           |
| 3.3          | 0.2737          | 0.9286          | 0.3003          | 0.2072          | 0.9542          | 0.2009          | 0.2558           | 0.941           | 0.2749          |
| 3.4          | 0.2822          | 0.9213          | 0.3068          | 0.2097          | 0.9523          | 0.2039          | 0.2634           | 0.935           | 0.2811          |
| 3.5          | 0.2901          | 0.9142          | 0.3127          | 0.2119          | 0.9505          | 0.2064          | 0.2701           | 0.9295          | 0.2864          |
| 3.6          | 0.2974          | 0.9075          | 0.318           | 0.2138          | 0.9489          | 0.2086          | 0.276            | 0.9246          | 0.2908          |
| 3.7          | 0.3039          | 0.9013          | 0.3226          | 0.2152          | 0.9475          | 0.2104          | 0.281            | 0.9203          | 0.2945          |
| 3.8          | 0.3096          | 0.8957          | 0.3267          | 0.2162          | 0.9464          | 0.2118          | 0.2852           | 0.9167          | 0.2973          |
| 3.9          | 0.3147          | 0.8908          | 0.3301          | 0.2169          | 0.9457          | 0.2129          | 0.2885           | 0.9139          | 0.2994          |
| 4.           | 0.3189          | 0.8867          | 0.3328          | 0.2172          | 0.9453          | 0.2136          | 0.291            | 0.9119          | 0.3007          |

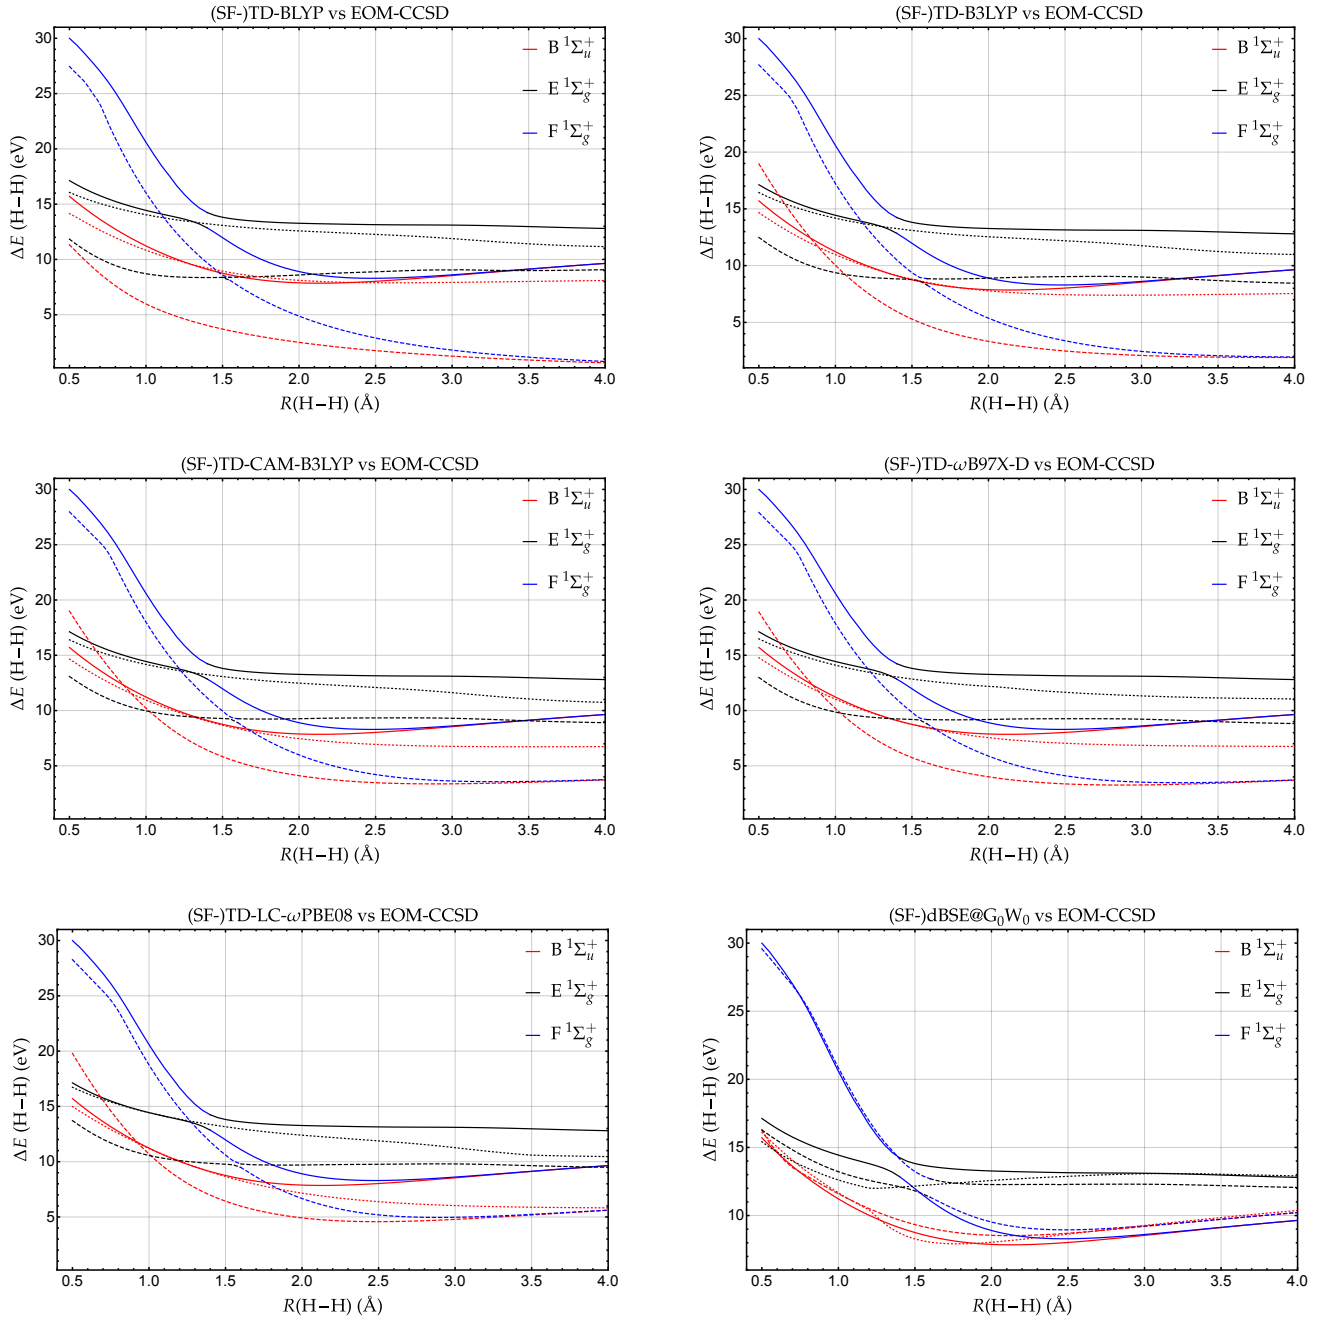

FIG. 1. Excitation energies with respect to the  $X^1\Sigma_g^+$  ground state of the  $B^1\Sigma_u^+$  (red),  $E^1\Sigma_g^+$  (black), and  $F^1\Sigma_g^+$  (blue) states of  $\text{H}_2$  obtained with the cc-pVQZ basis at various levels of theory. The reference EOM-CCSD excitation energies are represented as solid lines, while the results obtained with and without spin-flip are represented as dashed and dotted lines, respectively. All the spin-conserved and spin-flip calculations have been performed with an unrestricted reference.

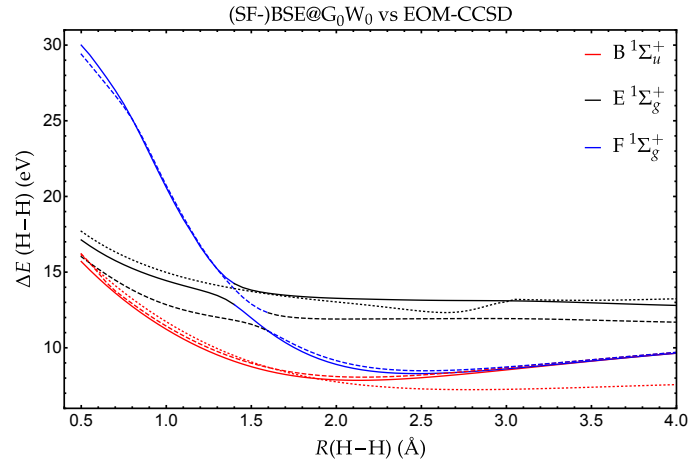

FIG. 2. Excitation energies with respect to the  $X^1\Sigma_g^+$  ground state of the  $B^1\Sigma_u^+$  (red),  $E^1\Sigma_g^+$  (black), and  $F^1\Sigma_g^+$  (blue) states of  $H_2$  obtained with the cc-pVQZ basis at the (SF-)BSE level of theory. The reference EOM-CCSD excitation energies are represented as solid lines, while the results obtained with and without spin-flip are represented as dashed and dotted lines, respectively. In this case, the spin-conserved calculations have been performed with a restricted reference while the spin-flip calculations have been performed with an unrestricted reference.
